# Supplementary material for: A Data-Centric Multi-Objective Learning Framework for Responsible Recommendation Systems
Source: arXiv:2310.13260 source file (2023-10-20)
Supplement: Supplementary file 1 [file appendix.tex]

\appendix

\section{Experiments} \label{sec:append}
We generate six solutions for each method in the four-objective scenario by setting MF-BPR and SASRec as backbone models respectively. The results are shown in Table~\ref{tab:appd_main_mf} and Table~\ref{tab:append_main_sasrec}. Solutions in Table~\ref{tab:main_mf}
 and Tabel~\ref{tab:append_main_sasrec} are selected from those solutions based on the strategy described in Section~\ref{RQ1}.

 From the performance of all solutions, similar findings could be concluded. MoRec outperforms baseline methods in term of average improvement across all objectives, and it regulates the drop of accuracy efficiently. Furthermore, solutions of MoRec are mostly not dominated by each other, demonstrating the Pareto efficiency remains in multiple objectives.

\begin{table*}[tbh]
\setlength{\abovecaptionskip}{2pt}
\setlength{\belowcaptionskip}{6pt}
\caption{Performance of all solutions over four objectives: MF-BPR ($\times 10^{-2}$).}
\label{tab:appd_main_mf}
\small
\begin{tabular}{@{}l|rrrrr|rrrrr|rrrrr@{}}
\toprule
Dataset & \multicolumn{5}{c|}{Electronics}   & \multicolumn{5}{c|}{Movies}        & \multicolumn{5}{c}{Xbox}           \\ \midrule
Metrics & Hit    & rHit   & Pop-KL & min-Hit & \textit{Imp} & Hit    & rHit   & Pop-KL & min-Hit & \textit{Imp} & Hit    & rHit   & Pop-KL & min-Hit & \textit{Imp} \\ \midrule
Base    & 1.62 & 135.42 & 142.54 & 0.91 & 0.00 & {4.09} & 112.68 & 83.11 & {3.57} & 0.00 & {20.27} & {532.53} & 51.94 & 3.28 & 0.00  \\ \midrule

\multirow{6}{*}{Static}  
& 1.62 & 197.56 & {37.09} & {1.00} & {32.41} & 4.06 & {136.92} & {27.74} & 2.16 & 11.99  & 18.22 & 681.73 & 4.93 & 3.68 & 30.16\\
& 1.23 & 248.08 & 7.92 & 0.05 & {14.59}  & 3.52 & 120.26 & 24.52 & 1.87 & 3.96 & 14.74 & 497.22 & 26.84 & 4.21 & 10.72 \\
& 0.99 & 189.72 & 12.52 & 0.14 & {14.59} &  3.74  & {176.93} & {6.14} & 2.02 & 24.42  & 16.62 & 507.10 & 15.84 & 10.80 & 69.05 \\
& 0.67 & 177.06 & 48.68 & 0.00 & {-15.53}  & 3.12 & 130.22 & 10.75 & 1.13 & 2.60  & 16.46 & 587.12 & 33.75 & 4.58 & 16.56 \\
& 1.31 & 229.77 & 2.61 & 0.14 & {20.95}  & 3.63 & 118.78 & 8.00 & 2.69 & 14.99  & 11.65 & 405.37 & 36.82 & 4.87 & 2.79\\
& 1.42 & 229.65 & 8.26 & 0.54 & {27.56}  & 2.64 & 125.22 & 32.16 & 1.99 & -1.80  & 8.81 & 286.42 & 19.09 & 0.19 & -33.44 \\ \midrule

\multirow{6}{*}{MGDA}    
& {1.32}  & {262.84}  & {20.37}  & 0.32 &  24.19  & 3.90  & {179.71} & 9.32 & 3.23 & 33.52 & 14.38  & 418.16 & {11.33} & 9.05 & 50.93 \\
& 1.28 & 256.53 & 19.74 &  0.25 & 20.52  & 3.87 & 179.17 & 9.42 & 3.19 & 32.87  & 14.32 & 419.91 & 11.00 & 8.93 & 50.18\\
& 1.29 & 252.07 & 19.63 & 0.29 & 20.86 & 3.85 & 177.63 & 9.26 & 3.21 & 32.65 & 14.32 & 418.47 & 11.38 & 9.07 & 51.01 \\
& 1.31 & 255.88 & 20.07 & 0.29 & 21.72 & 3.88 & 180.09 & 9.33 & 3.25 & 33.62  & 14.31 & 416.84 & 11.38 & 9.39 & 53.37\\
& 1.28 & 256.53 & 19.74 & 0.25 & 20.52  & 3.83 & 176.97 & 9.51 & 3.18 & 32.10  & 14.27 & 420.14 & 11.43 & 9.11 & 51.30\\
& 1.26 & 254.74 & 20.21 & 0.36 & 22.74  & 3.89 & 179.57 & 8.87 & 3.22 & 33.47  & 14.22 & 418.03 & 11.28 & 8.77 & 48.61
\\ \midrule

\multirow{6}{*}{PEMTL} 
& 1.68 &  {167.53} & {99.08} &  {1.03}  &  17.60  & 4.08 & 161.25 & 9.09 & 3.10 & 29.70  & 17.54 & 679.04 & 6.34 & 3.37 & 26.17\\
& 1.26  &  {245.74} & {9.12} &  0.32  &  22.00  & 3.92  & 176.61 & {8.54} & 3.20 & 32.94 & 14.47 & 398.90 & 14.24 & 10.42 & 59.17 \\
& 1.50 & 89.10 & 87.11 & 0.95  & 0.28 & 3.88 & 98.26 & 41.24 & 3.05 & 4.44  & 14.31 & 376.86 & 23.61 & 9.53 & 46.68\\
& 1.51 & 89.95 & 103.67 & 0.90 & -3.59  & 4.20 & 161.96 & 21.01 & 3.10 & 26.96  & 8.85 & 272.77 & 49.18 & 3.22 & -25.39\\
& 1.53 & 86.61 & 124.73 & 0.94 & -6.54  & 3.71 & 96.36 & 0.75 & 2.96 & 14.55  & 10.62 & 188.17 & 12.43 & 7.40 & 22.39\\
& 1.28 & 242.86 & 15.34 & 0.32 & 22.00  & 3.62 & 161.03 & 0.34 & 2.70 & 26.66  & 8.08 & 274.40 & 59.12 & 4.06 & -24.63\\ \midrule

\multirow{6}{*}{EPO} 
 & 1.51 & 162.99 & 35.75 & 0.98 & 23.83  & 3.97 & 160.46 & 9.14 & 2.44 & 24.22 & 16.89 & 645.64 & 3.89 & 4.90 & 36.67 \\
& 1.27  &  {229.45} &  {6.48}  &  0.50 &  24.46   & 4.09 & 127.06 & 26.29 & 3.30 & 18.38   & 8.52 & 301.91 & 32.23 & 0.22 & -39.12 \\
 & 1.13 & 164.46 & 0.42 & 0.58 & 13.68  & 3.76 & 125.72 & 0.22 & 2.30 & 16.90  & 14.74 & 580.28 & 35.42 & 6.27 & 26.21\\
 & 1.19 & 217.59 & 3.29 & 0.00 & 7.86 &  2.78 & 119.82 & 2.53 & 0.14 & -6.18  & 15.55 & 503.49 & 13.26 & 10.57 & 67.07\\
 & 1.46 & 164.38 & 23.20 & 0.91 & 23.74 & 3.82 & 136.43 & 18.27 & 2.35 & 14.61 & 12.47 & 567.83 & 11.35 & 5.27 & 26.78 \\
 & 1.22 & 210.48 & 2.70 & 0.48 & 20.31 & 2.93 & 124.58 & 23.59 & 2.49 & 5.90  & 9.74 & 351.23 & 57.70 & 3.60 & -21.81\\ \midrule

\multirow{6}{*}{MoRec} 
& {1.63} &  {225.19}  &  {16.81}  &  {1.05}  &    {42.60} & {3.98} &  164.44 &  9.73 & {3.68} & {33.69} &  {19.71}  & {575.66} & 18.52 & {11.98} & {83.79} \\
 & 1.59 & 223.12 & 23.35 & 1.09 & 41.40 & 4.26 & 164.31 & 19.56 & 3.67 & 32.32 & 19.14 & 584.79 & 10.32 & 10.28 & 74.47\\
 & 1.61 & 176.48 & 85.58 & 1.12 & 23.13 & 4.12 & 159.24 & 10.68 & 3.70 & 33.23 & 19.21 & 554.59 & 20.97 & 9.27 & 60.34\\
 & 1.59 & 166.36 & 32.07 & 1.27 & 34.45 & 4.05 & 158.68 & 7.56 & 3.71 & 33.65 & 19.41 & 626.71 & 4.91 & 8.55 & 66.19 \\
 & 1.59 & 196.59 & 20.09 & 1.24 & 41.25&3.99 & 162.53 & 11.59 & 3.67 & 32.61   & 19.71 & 575.66 & 18.52 & 11.98 & 83.79 \\
 & 1.63 & 162.01 & 7.11 & 1.06 & 32.90&4.03 & 155.43 & 10.74 & 3.87 & 32.99  & 19.94 & 642.92 & 6.83 & 7.80 & 61.00\\
\bottomrule
\end{tabular}
\end{table*}

\begin{table*}[thb]
\caption{Performance of all solutions over four objectives: SASRec-BCE ($\times 10^{-2}$).} 
\label{tab:append_main_sasrec}
\small
\centering
\begin{tabular}{@{}l|rrrrr|rrrrr|rrrrr@{}}
\toprule
Dataset & \multicolumn{5}{c|}{Electronics}   & \multicolumn{5}{c|}{Movies}        & \multicolumn{5}{c}{Xbox}           \\ \midrule
Metrics & Hit    & rHit   & pop-kl & min-Hit & \textit{Imp} & Hit    & rHit   & pop-kl & min-Hit & \textit{Imp} & Hit    & rHit   & pop-kl & min-Hit & \textit{Imp} \\ \midrule
Base    & 1.81 & 174.53 & 26.38 & 0.75 & 0.00 &  {5.93} &  {175.17} & 10.78 & 4.13 &  {0.00}  & \textbf{25.99} & 809.74 &  {17.16} & 7.84 & 0.00  \\\midrule

\multirow{6}{*}{Static} 
& 1.84 & 259.75 & 20.49 & 0.40 & 6.51 & 5.21 & 163.30 & 8.63 & 3.24 & -5.16 & 13.73 & 700.68 & 32.45 & 0.67 & -60.30\\
& 1.50 & 295.59 & 18.49 & 0.07 & -2.27 & 4.19 & 185.59 & 19.27 & 3.94 & -26.70 & 12.87 & 628.82 & 110.90 & 1.25 & -175.83\\
& 1.31 & 355.52 & 16.33 & 0.02 & 4.24 & 2.14 & 67.65 & 134.30 & 1.89 & -331.38 & 13.67 & 676.92 & 113.94 & 0.97 & -178.90\\
& 0.79 & 95.10 & 157.05 & 0.07 & -172.03 & 1.71 & 79.63 & 27.79 & 0.56 & -92.47 & 11.67 & 600.18 & 130.25 & 0.63 & -208.03\\
& 0.96 & 251.61 & 37.84 & 0.11 & -32.87 & 3.85 & 145.96 & 18.10 & 2.72 & -38.46 & 11.01 & 447.41 & 148.85 & 1.57 & -237.49\\
& 1.62 & 249.50 & 39.21 & 0.13 & -24.66 & 4.82 & 152.40 & 15.75 & 3.80 & -21.48 & 9.84 & 393.02 & 159.76 & 1.72 & -255.71 \\ \midrule

\multirow{6}{*}{MGDA} 
& 1.70 & 175.00 & 42.23 & 0.37 & -29.30 & 5.50 & 167.22 & 14.34 & 4.57 & -8.50 & 25.66 & 932.78 & 20.88 & 8.46 & 0.04\\
& 1.59 & 166.06 & 43.18 & 0.31 & -35.01 & 5.34 & 159.11 & 15.44 & 4.42 & -13.85 & 24.32 & 878.34 & 29.58 & 8.92 & -14.13\\
& 1.56 & 162.84 & 44.02 & 0.17 & -41.19 & 5.33 & 162.77 & 16.28 & 4.37 & -15.64 & 25.05 & 899.42 & 19.85 & 8.53 & 0.14\\
& 1.61 & 167.41 & 44.25 & 0.29 & -36.01 & 5.30 & 162.28 & 15.72 & 4.23 & -15.32 & 24.96 & 912.27 & 24.09 & 8.42 & -6.05\\
& 1.64 & 165.32 & 44.15 & 0.40 & -32.29 & 5.50 & 167.22 & 14.34 & 4.57 & -8.50 & 24.92 & 887.37 & 22.41 & 8.73 & -3.44\\
& 1.60 & 175.17 & 45.82 & 0.23 & -38.65 & 5.41 & 160.55 & 15.48 & 4.49 & -12.99 & 24.53 & 913.75 & 23.77 & 8.56 & -5.53\\ \midrule

\multirow{6}{*}{PEMTL}
& 2.46 & 220.91 & 45.40 & 1.28 & 15.10 & 5.81 & 153.64 & 14.69 & 4.08 & -12.94 & 25.41 & 812.74 & 32.84 & 9.63 & -17.58\\
& 1.25 & 332.29 & 27.58 & 0.05 & -9.80 & 5.83 & 151.29 & 16.51 & 2.63 & -26.24 & 18.43 & 376.06 & 27.79 & 8.27 & -34.78\\
& 1.58 & 165.69 & 43.18 & 0.35 & -33.64 & 4.05 & 191.27 & 26.98 & 3.25 & -48.51 & 19.88 & 960.85 & 36.78 & 2.12 & -48.04\\
& 1.64 & 112.16 & 45.96 & 0.50 & -38.06 & 5.09 & 153.03 & 15.89 & 4.08 & -18.86 & 24.30 & 892.57 & 27.09 & 8.05 & -12.87\\
& 1.94 & 112.72 & 29.32 & 1.02 & -0.71 & 6.02 & 156.25 & 19.23 & 2.72 & -30.44 & 25.10 & 822.56 & 25.44 & 9.42 & -7.48\\
& 0.51 & 40.51 & 276.65 & 0.06 & -297.26 & 5.17 & 143.12 & 43.87 & 3.87 & -86.08 & 22.58 & 950.25 & 32.58 & 5.27 & -29.59\\ \midrule

\multirow{6}{*}{EPO}
& 1.69 & 228.42 & 43.57 & 0.31 & -25.04 & 5.15 & 157.85 & 18.05 & 3.24 & -28.02 & 21.12 & 995.70 & 47.42 & 2.03 & -61.57\\
& 1.31 & 238.97 & 24.44 & 0.02 & -20.15 & 4.23 & 185.92 & 27.58 & 3.38 & -49.14 & 12.46 & 639.65 & 119.58 & 0.52 & -190.86\\
& 0.84 & 100.88 & 180.92 & 0.05 & -193.94 & 2.21 & 70.62 & 152.64 & 1.93 & -372.96 & 19.61 & 766.05 & 70.58 & 4.19 & -96.96\\
& 1.14 & 250.75 & 42.05 & 0.12 & -34.16 & 1.92 & 88.86 & 24.72 & 0.28 & -84.86 & 11.98 & 447.65 & 104.38 & 0.04 & -176.64\\
& 1.34 & 197.83 & 52.78 & 0.09 & -50.13 & 4.87 & 174.38 & 21.79 & 3.48 & -34.08 & 20.57 & 897.84 & 68.31 & 4.99 & -86.10\\
& 1.58 & 214.71 & 69.19 & 0.05 & -61.34 & 5.02 & 186.24 & 47.36 & 3.72 & -89.56 & 15.85 & 977.32 & 95.57 & 2.76 & -135.05\\ \midrule

\multirow{6}{*}{MoRec}
& 2.32 & 239.54 & 14.87 & 1.47 & 51.38 & 6.25 & 189.26 & 1.64 & 5.17 & 30.84 & 25.96 & 899.47 & 7.64 & 14.12 & 36.65 \\
& 2.11 & 275.37 & 16.76 & 1.15 & 41.17 & 5.80 & 203.36 & 7.24 & 4.34 & 12.95 & 24.40 & 865.28 & 11.62 & 12.28 & 22.42 \\
& 2.31 & 227.94 & 5.94 & 1.26 & 51.08 & 5.88 & 171.11 & 7.06 & 4.45 & 9.76 & 24.00 & 749.38 & 16.34 & 9.61 & 3.06 \\
& 2.10 & 255.92 & 14.18 & 1.24 & 43.62 & 6.01 & 196.10 & 4.65 & 4.70 & 21.01 & 23.62 & 820.82 & 18.69 & 10.03 & 2.84 \\
& 2.04 & 204.69 & 15.48 & 1.50 & 42.76 & 5.91 & 178.59 & 3.08 & 5.03 & 23.75 & 25.53 & 893.94 & 8.64 & 14.31 & 35.23 \\
& 2.22 & 218.56 & 11.31 & 1.48 & 50.45 & 5.96 & 195.73 & 9.25 & 5.29 & 13.63 & 23.67 & 855.87 & 15.62 & 11.23 & 12.27 \\
\bottomrule
\end{tabular}
\end{table*}

% \subsection{Sensitivity w.r.t Number of Groups}
